# Supplementary material for: EarthNet2021: A novel large-scale dataset and challenge for forecasting localized climate impacts
Source: arXiv:2012.06246 source file (2020-12-11)
Supplement: Supplementary file 1 [file 06supplementary.tex]

\begin{appendices}
\label{par:suplementary}

\section{EarthNet2021 dataset generation}
\label{par:datagen}

EarthNet2021 evolved from a complex procedure merging Sentinel 2 satellite imagery, E-OBS climatic conditions and EU-DEM digital surface model. In the following paragraphs we describe the complete procedure by which the dataset was generated. 

\subsection{Sentinel 2}

\paragraph{Metadata-based pre-filtering.} 
We obtain Sentinel 2 satellite imagery from the AWS Open Data Registry\footnote{\url{https://registry.opendata.aws/sentinel-2/}}. Because the data there lays in so-called requester pays buckets and downloading Terabytes of data takes time, we first obtain metadata to pre-filter which tiles to download. We use the sentinelhub library\footnote{\url{https://sentinelhub-py.readthedocs.io/en/latest/}} for downloading \emph{tileinfo} and \emph{metadata} files, which are freely available. These files allow us to extract quality information regarding the data coverage, cloudiness and the amount of pixels classified by Sen2Cor\footnote{\url{http://step.esa.int/main/third-party-plugins-2/sen2cor/}} as water. We collect this metadata for all Sentinel 2 takes shot between Nov. 1st 2016 and June 1st 2020 over the area from 12\degree west to 24\degree east and from 36\degree to 64\degree north. This roughly covers Europe.

Sentinel 2 is available over the military grid reference system, which cuts the world up in tiles. In general, each tile is covered every 5 days. Because of overlap, in practice it is covered more frequently but under varying off-nadir angles. To keep the off-nadir angle low and constant within a certain tile, we determine the 5-day interval with the highest data coverage. After filtering by this, we have a timeseries of metadata over 5-day intervals for each sentinel tile. We generate the final list of tiles to download by filtering out tiles covering less than 20\% of land (on the least-cloudy day) and those with less than 90\% of data coverage.

\paragraph{Subsampling, tile download.}
From the final list of tiles we take a random sample of size 110. For these we download Bands B02, B03, B04, B8A, CLD and SCL using sentinelhub.

\paragraph{Co-registration via arosics.}
We notice a bit of jittering between consecutive Sentinel 2 takes, probably resulting from the two satellites used not being perfectly aligned. We try to compensate this by co-registering the timeseries of each tile. We use the global co-registration from the arosics library\footnote{\url{https://pypi.org/project/arosics/}} \citep{scheffler2017} inside a custom loop. More specifically, for each tile we take the least-cloudy frame as reference. We register all the other tiles to the reference by using arosics' global co-registration over all possible windows of size 512x512px until it finds a calculated shift within feasible boundaries (maximum 3 pixel). Tiles are interpolated bicubic, except for CLD and SCL layers, which are interpolated by nearest-neighbour.

\subsection{Data Fusion}
Each Sentinel 2 tile is individually merged with the other predictors in EarthNet2021.

\paragraph{E-OBS climatic variables.}
We download E-OBS\footnote{\url{https://surfobs.climate.copernicus.eu/dataaccess/access_eobs.php}} climatic varibles daily mean temperature TG, daily minimum temperature TN, daily maximum temperature TX, daily precipitation sum RR and daily averaged sea level pressure PP. We merge the long-term E-OBS dataset with the latest months until May 2020.

\paragraph{EU-DEM surface model.}
We download the EU-DEM\footnote{\url{https://www.eea.europa.eu/data-and-maps/data/eu-dem}} over full Europe. The extent of the DEM has been the limiting factor for the intake window from which we have considered Sentinel 2 tiles.

\paragraph{Reproject, resample \& cut.}
We calculate a meso-scale window, which allows us to later extract predictors outside of each individual Sentinel 2 take. We reproject the climatic variables and the DEM to this meso-scale window. Additionally we reproject the DEM to the high-resolution window of the Sentinel 2 take. Meso-scale variables are resampled using bilinear interpolation to match a 1.28km ground resolution. The high-resolution DEM is resampled using bilinear interpolation to match the 20m ground resolution of the Sentinel 2 tiles.

\subsection{Cube generation.}
We calculate geolocations for the multicubes for each Sentinel 2 tile. These geolocations are chosen such that in the end the high-resolution data of size 2.56x2.56km (128x128px) covers the central 2x2px of the meso-scale data of size 102.4x102.4km (80x80px). The high-resolution data of different geolocations is non-overlapping, while the meso-scale data might overlap. The following steps are performed for each such geolocation.

\paragraph{Creating data quality mask.}
Leveraging the scene classification layer of Sentinel 2, we create a data quality mask. All pixels without data are masked, additionally all pixels where the sum of the RGB channels is bigger than 0.435 and the blue channel plus 0.03 is bigger than the green channel. Additionally all pixels where the blue channel is bigger than 0.35 are masked. Also all pixels where the scene classification layer shows them as being no data, saturated / defective, dark area pixels, cloud shadows, clouds low probability, clouds medium probability, clouds high probability or cirrus are masked. Finally the whole mask is eroded by a 3x3 kernel and then dilated by a 7x7 kernel. This removes very small artifacts and then smooths the masks at the borders. The whole process is motivated by the idea that for the calculation of EarthNetScore it is better if the mask is over-restrictive than if it leaves out clouds. Also, it is in line with the work of \citet{meraner2020}. Still, the data quality mask is far from being perfect.

\paragraph{Saving compressed array.}
The multicube is saved as a compressed numpy array. It contains the following arrays:
\begin{itemize}
    \item highresdynamic (shape 128x128x7xt)
    \item mesodynamic (shape 80x80x5x(t*5))
    \item highresstatic (shape 128x128)
    \item mesostatic (shape 80x80)
\end{itemize}

\paragraph{Saving data quality table.}
For each multicube we generate a set of data quality indicators. These are collected over all multicubes and then saved to a data quality table.

\subsection{Dataset split.}
Up until this point, we have generated over 1.4 million multicubes. Many of which are not useful for neither training nor evaluating deep learning models because they are too cloudy. Also, we have to split the data into training and test sets.

\paragraph{Quality vs. Bias trade-off.}
Whenever we filter data in order to keep only high-quality data we likely impose certain biases. We would like models developed using EarthNet2021 to be able to work over full Europe. Thus we carefully tackle the quality vs. bias trade-off by both requiring certain minimum quality and that the dataset is minimum a bit diverse in certain criteria.

We achieve this by calcuting a quality score as
\begin{align*}
    QS =& \frac{cd_{10}+mcd_{10}+d_{10}+cd_{50}+mcd_{50}+d_{50}+cd_{90}+mcd_{90}+d_{90}}{30} \\ 
    &- log(max(1-\varepsilon, 1-w)) \\
    &- log(max(1-\varepsilon, 1-apct^{0.25})) \\
    &+ 2*pct^2  
\end{align*}
where $\varepsilon$ is $1e-8$, $cd_x$ is the number of context days over x\% masked, $mcd_x$ is the maximum number of consecutive days over x\% masked, $d_x$ is the number of days over x\% masked, $w$ is the maximal percentage of pixels that are water in a frame, $apct$ is the percentage of pixels that are always masked in the context frames and $pct$ is the total percentage of pixels masked. We set a quality restriction $x$. For each tile, we filter out multicubes with more than 15 days over 70\% masked, more than 5 context days over 70\% masked, more than 50\% of pixels as water, at least 40\% of total pixels masked or more than 5 consecutive days over 70\% masked. The remaining set we sort by quality score $QS$ and we take the best $x*l$ multicubes, where $l$ is the number of multicubes for the tile before filtering, but not more than 1500 multicubes per tile.

Then we calculate the maximum number of cubes per starting month. For each starting month we check, if at least half the maximum number of cubes are still included. If not, we fill that month with cubes that follow the same quality criteria as mentioned above, again sorted by quality score $QS$. Also, we check if at least 10000 multicubes are located in the northern 50\% of the study extent. If this is not the case, we fill up in the same way as above. We iteratively loosen quality restriction $x$ until we have at least 32000 multicubes.
        
\paragraph{Iterative sampling process.}
The step above left us with a dataset corpus of 32337 multicubes. From these we iteratively obtain the OOD set by randomly sampling 16 tiles and then checking the multicubes belong to these tiles in the dataset corpus. We accept the choice if between 4000 and 4500 multicubes are in the OOD test set and of them at least 1500 are in the norther 50\% of the study extent. Otherwise we sample again. The remaining cubes are randomly split into the training and IID test sets.

\paragraph{Train and four test sets.}
The resulting training set has 23904 cubes, the IID test set 4219 cubes and the OOD test set 4214 cubes. For the extreme summer test set, which is over the four tiles 32UMC, 32UNC, 32UPC, 32UQC (we excluded multicubes from these locations from the years 2018, 2019 and 2020 from the training, IID and OOD test sets), we first have to generate the multicubes. These encompass from February to November 2018, over 60 frames in total. We then filter out multicubes with more than 50\% water or more than 1\% of pixels always masked in the context frames. We then take the best 300 cubes per tile sorted by total percentage of pixels masked. Out of this set we take the best 4000 cubes by total percentage of pixels masked. We perform the same procedure for the seasonal cycle test set. In this case, multicubes start in June 2017 and extend for 210 frames (3 years).

\section{EarthNetScore}
\label{par:ENS}

\paragraph{Basic concept.}
The EarthNetScore shall provide a ranking between different predictions based on components covering the distance of values, the similarity of pixelwise timeseries and the perceptual plausibility. Its computation builds upon subscores calculated for each multicube in a test set. The full test set EarthNetScore is then computed by aggregating all of these, as described later. It is also possible to compute the EarthNetScore for a single predicted multicube. 
For a single cube, the EarthNetScore takes the target cube $T \in [0,1]^{t,c,h,w}$, the predicted cube $P \in [0,1]^{t,c,h,w}$ and a binary quality mask $M \in \{0,1\}^{t,c,h,w}$ with dimensions time, channel, height, and width as inputs. The EarthNetScore is computed as
\begin{align*}
    ENS(T,M,P) = \frac{4}{(\frac{1}{MAD(T,M,P)} + \frac{1}{OLS(T,M,P)} + \frac{1}{EMD(T,M,P)} + \frac{1}{SSIM(T,M,P)})}\,,
\end{align*}
here $MAD$, $OLS$, $EMD$ and $SSIM$ are the component scores described in the following. We chose the harmonic mean for aggregating the four subscores since it is always the lowest of the pythagorean means and thus requires predictions to be good in all four metrics. For this to be true, the four subscores must be somehow equally difficult, i.e., in a similar range. While not perfectly solving this task, we rescale subscores so that the ranking criterion gets better, as described later.

\paragraph{Median absolute deviation score.}
The median absolute deviation score $MAD$ is computed on the flattened arrays $P$ and $T$ at non-masked values. For these values the median absolute deviation $mad$ is calculated. Then, $MAD = 1-mad$, its values are from 0 (worst) to 1 (best).

\paragraph{Ordinary least squares score.}
The ordinary least squares score $OLS$ is computed between predicted and target NDVI. For each pixelwise timeseries, the ordinary least squares slope (on the regressor time) is calculated. Target slopes are calculated over all non-masked values. Predicted slopes are calculated over all values laying between the minimum and maximum non-masked timestep. The regressors for both slopes are independently rescaled, such that the resulting slopes lie between -1 and 1. Slopes are only calculated if at least two datapoints are available. For slopes $b_{pred}$ and $b_{targ}$ the distance $ols = \frac{abs(b_{pred} - b_{targ})}{2}$ is used for the computation of the score $OLS = 1-mean(ols)$, its values are from 0 (worst) to 1 (best). The computation of $OLS$ is completely implemented as matrix operations in NumPy using broadcasting and thus computationally efficient.

\paragraph{Earth mover distance score.}
The earth mover distance score $EMD$ is based on the wasserstein-1 distance between predicted and target pixelwise NDVI timeseries distributions. For each such distribution, the wasserstein-1 distance $w1$ is computed between non-masked target values and all predicted values. Then, the score is $EMD = 1-mean(w1)$, its values are from 0 (worst) to 1 (best). The computation of $EMD$ can not be implemented as only matrix operations, but is still fast as $w1$ computation for 1d distributions is cheap.

\paragraph{Structural similarity index score.}
The structural similarity index score $SSIM$ is computed on the full spatial image, each channel and timestep is treated as an individual frame. For each frame, if the target is less than 30\% masked, the SSIM is computed, masked pixels of the target frame are replaced with the corresponding pixels from the prediction. $SSIM$ is then the mean of all SSIM over all frames, its values lay between 0 (worst) and 1 (best).

\paragraph{Treatment of missing data.}
Throughout subscore computation, missing data is usually handled by performing all aggregation methods in such a way that the missing datapoints are ignored. It is possible (but very rare) though, that during computation no valid datapoint is available. Then the respective score is returned to be \emph{NaN} and during computation of the EarthNetScore for this cube, the particular score is not considered in the harmonic mean.

\paragraph{Subscore rescaling.}
Subscores represent model skill in a certain area and should be comparable to each other so that it is not easy to cheat EarthNetScore by specialising on the score that is scaled the lowest. Of course it is a difficult endeavour to properly rescale subscores. Our approach is to take as reference expected worst-case scores for $MAD$, $OLS$ and $EMD$ and an intuitive requirement for $SSIM$. All subscores are rescaled so that the reference points achieve a subscore of $0.1$. More specifically for $MAD$ we compute the size of a 99.7\% confidence interval from the variance of the pixelwise centered timeseries (of bands R,G,B,NIR) in the EarthNet2021 training set. We understand this as a proxy for a maximally plausible distance for two values belonging to the same distribution. Thus if models randomly pick values from this distribution, they maximally would end up with this value. Using basic algebra we obtain a scaling factor of $sf_{mad} = 0.06649346971087526$, that is applied by $mad = mad^{sf_{mad}}$. Similarly, for $OLS$ and $EMD$ we get scaling factors by computing the size of a 99.7\% confidence interval from the variance of the pixelwise centered NDVI timeseries in the EarthNet2021 training set. We get $sf_{ndvi} = 0.10082047548620601$ and apply it to $ols = ols^{sf_{ndvi}}$ and $w1 = w1^{sf_{ndvi}}$. Finally $SSIM$ is rescaled by a scaling factor $sf_{SSIM} = 10.31885115$. This factor sets a $SSIM = 0.8$ to $SSIM = 0.1$, thus requiring models to perceptually achieve at least a decent quality (here defined by us as a score of $0.8$). With this rescaling we also allow for more headroom to compare models without having to dissect decimal places.

\paragraph{Composition of dataset EarthNetScore.}
Computing EarthNetScore $ENS$ over a full dataset is done by
\begin{enumerate}
    \item calculating the four components $MAD, OLS, EMD, SSIM$ for each cube,
    \item taking the arithmetic mean over cubes per subscore,
    \item taking the harmonic mean over the four subscores.
\end{enumerate}
If instead of one prediction per cube, a stochastic model has generated multiple predictions. Then for each cube a single prediction is picked by taking the single prediction for that cube that has the highest EarthNetScore. The arithmetic mean of the subscores, of course, ignores NaNs, so missing data. For the very unlikely case that one of the arithmetic means turns out to be NaN, this mean is ignored in the harmonic mean.

\section{Tools}
The following tools have been used:
\begin{itemize}
    \item General: Numpy \citep{harris2020}, Scipy \citep{virtanen2020}, Matplotlib \citep{hunter2007}, Pandas \citep{mckinney2011}, Cartopy\footnote{\url{https://scitools.org.uk/cartopy/docs/latest/}}
    \item Dataset generation: GDAL\footnote{\url{https://gdal.org}}, Arosics \citep{scheffler2017}, Sentinelhub\footnote{\url{https://sentinelhub-py.readthedocs.io/en/latest/}}
    \item Evaluation: Scikit-image \citep{van2014}, Seaborn\footnote{\url{https://seaborn.pydata.org/}}
    %\item Manuscript writing: Overleaf hosted by GWDG\footnote{\url{https://sharelatex.gwdg.de/}}, Mayavi \citep{ramachandran2011}, Microsoft PowerPoint, Adobe Photoshop
\end{itemize}

\end{appendices}
